# Supplementary material for: An observational determination of the evolving extragalactic background light from the multiwavelength HST/CANDELS survey in the Fermi and CTA era
Source: arXiv:2012.03035 source file (2021-09-28)
Supplement: Supplementary file 1 [file A_appendix.tex]

\newpage
\section{CANDELS Photometry Data Set}\label{appA}
\autoref{tab:candels_bands} contains a summary of all the obeserved photometric bands by the CANDELS program (see Sect.\ \ref{sec:data} and the references wherein). Additional GALEX, \emph{Spitzer} and Herchel photometry are also presented. The chart is sorted by the corresponding instrument and filter central wavelength, which is given in angstroms (\AA).

\begin{table*}
\caption{Summary of photometric broad- and intermediate-band data set available in \emph{Rainbow Navigator} for the 5 CANDELS fields.}
\begin{tabular}{cccccccc}
%\hline
Instrument & Filter & $\mathrm{\lambda}$ (\AA) & GOODS--S & UDS & COSMOS & EGS & GOODS--N \\
\hline
GALEX & FUV & 1538 & \checkmark & -- & -- & -- & \checkmark \\
GALEX & NUV & 2315 & \checkmark & -- & -- & -- & \checkmark \\
Blanco/MOSAIC--II & U\_CTIO & 3734 & \checkmark & -- & -- & -- & -- \\
VLT/VIMOS & U\_VIMOS & 3722 & \checkmark & -- & -- & -- & -- \\
KPNO4m/Mosaic & U & 3592 & -- & -- & -- & -- & \checkmark \\
LBT/LBC & U$^{/}$ & 3633 & -- & -- & -- & -- & \checkmark \\
CFHT/MegaPrime & u & 3817 & -- & -- & \checkmark & -- & -- \\
CFHT/MegaPrime & g & 4317 & -- & -- & \checkmark & -- & -- \\
CFHT/MegaPrime & r & 6220 & -- & -- & \checkmark & -- & -- \\
CFHT/MegaPrime & i & 7606 & -- & -- & \checkmark & -- & -- \\
CFHT/MegaPrime & z & 8816 & -- & -- & \checkmark & -- & -- \\
CFHT/MegaCam & u$^{*}$ & 3860 & -- & \checkmark & -- & \checkmark & -- \\
CFHT/MegaCam & g$^{/}$ & 4890 & -- & -- & -- & \checkmark & -- \\
CFHT/MegaCam & r$^{/}$ & 6250 & -- & -- & -- & \checkmark & -- \\
CFHT/MegaCam & i$^{/}$ & 7690 & -- & -- & -- & \checkmark & -- \\
CFHT/MegaCam & z$^{/}$ & 8880 & -- & -- & -- & \checkmark & -- \\
CFHT/MegaCam & K & 213470 & -- & -- & -- & -- & \checkmark \\
Subaru/Suprime--Cam & B & 4448 & -- & \checkmark & \checkmark & -- & -- \\
Subaru/Suprime--Cam & g$^{+}$ & 4761 & -- & -- & \checkmark & -- & -- \\
Subaru/Suprime--Cam & V & 5470 & -- & \checkmark & \checkmark & -- & -- \\
Subaru/Suprime--Cam & r$^{+}$ & 6276 & -- & -- & \checkmark & -- & -- \\
Subaru/Suprime--Cam & R$_c$ & 6500 & -- & \checkmark & -- & -- & -- \\
Subaru/Suprime--Cam & i$^{+}$ & 7671 & -- & \checkmark & \checkmark & -- & -- \\
Subaru/Suprime--Cam & z$^{+}$ & 9096 & -- & \checkmark & \checkmark & -- & -- \\
Subaru/MOIRCS & K$_{s}$ & 21577 & -- & -- & -- & -- & \checkmark \\
HST/ACS & F435W & 4317 & \checkmark & -- & -- & -- & -- \\
HST/ACS & F606W & 5918 & \checkmark & \checkmark & \checkmark & \checkmark & \checkmark \\
HST/ACS & F775W & 7693 & \checkmark & -- & -- & -- & \checkmark \\
HST/ACS & F814W & 8047 & \checkmark & \checkmark & \checkmark & \checkmark & \checkmark \\
HST/ACS & F850LP & 9055 & \checkmark & -- & -- & -- & \checkmark \\
HST/WFC3 & F098M & 9851 & \checkmark & -- & -- & -- & -- \\
HST/WFC3 & F105W & 10550 & \checkmark & -- & -- & -- & \checkmark \\
HST/WFC3 & F125W & 12486 & \checkmark & \checkmark & \checkmark & -- & \checkmark \\
HST/WFC3 & F140W & 13970 & -- & -- & -- & \checkmark & \checkmark \\
HST/WFC3 & F160W & 15370 & \checkmark & \checkmark & \checkmark & \checkmark & \checkmark \\
VISTA/VIRCAM & Y & 10210 & -- & -- & \checkmark & -- & -- \\
VISTA/VIRCAM & J & 12524 & -- & -- & \checkmark & -- & -- \\
VISTA/VIRCAM & H & 16431 & -- & -- & \checkmark & -- & -- \\
VISTA/VIRCAM & Ks & 21521 & -- & -- & \checkmark & -- & -- \\
VLT/ISAAC & Ks & 21605 & \checkmark & -- & -- & -- & -- \\
UKIRT/WFCAM & J & 12510 & -- & \checkmark & -- & -- & -- \\
UKIRT/WFCAM & H & 16360 & -- & \checkmark & -- & -- & -- \\
UKIRT/WFCAM & K & 22060 & -- & \checkmark & -- & -- & -- \\
Mayall/NEWFIRM & J1 & 10470 & -- & -- & \checkmark & \checkmark & -- \\
Mayall/NEWFIRM & J2 & 11950 & -- & -- & \checkmark & \checkmark & -- \\
Mayall/NEWFIRM & J3 & 12790 & -- & -- & \checkmark & \checkmark & -- \\
Mayall/NEWFIRM & H1 & 15610 & -- & -- & \checkmark & \checkmark & -- \\
Mayall/NEWFIRM & H2 & 17070 & -- & -- & \checkmark & \checkmark & -- \\
Mayall/NEWFIRM & K & 21700 & -- & -- & \checkmark & \checkmark & -- \\
CHFT/WIRCAM & J & 12540 & -- & -- & -- & \checkmark & -- \\
CHFT/WIRCAM & H & 16360 & -- & -- & -- & \checkmark & -- \\
CHFT/WIRCAM & Ks & 21590 & -- & -- & -- & \checkmark & -- \\
VLT/HAWK--1 & Y & 10190 & -- & \checkmark & -- & -- & -- \\
VLT/HAWK--1 & Ks & 21463 & \checkmark & \checkmark & -- & -- & -- \\
Spitzer/IRAC & 3.6~$\mu$m & 35508 & \checkmark & \checkmark & \checkmark & \checkmark & \checkmark \\
Spitzer/IRAC & 4.5~$\mu$m & 44960 & \checkmark & \checkmark & \checkmark & \checkmark & \checkmark \\
Spitzer/IRAC & 5.8~$\mu$m & 57245 & \checkmark & \checkmark & \checkmark & \checkmark & \checkmark \\
Spitzer/IRAC & 8.0~$\mu$m & 78840 & \checkmark & \checkmark & \checkmark & \checkmark & \checkmark \\
Spitzer/MIPS & MIPS/24 & 238440 & \checkmark & \checkmark & \checkmark & \checkmark & \checkmark \\
Spitzer/MIPS & MIPS/70 & 724936 & \checkmark & \checkmark & \checkmark & \checkmark & \checkmark \\
Herschel/PACS & PACS/100 & 1022522 & \checkmark & \checkmark & \checkmark & \checkmark & \checkmark \\
Herschel/PACS & PACS/160 & 1656067 & \checkmark & \checkmark & \checkmark & \checkmark & \checkmark \\
Herschel/SPIRE & SPIRE/250 & 2531298 & \checkmark & \checkmark & \checkmark & \checkmark & \checkmark \\
Herschel/SPIRE & SPIRE/350 & 3558741 & \checkmark & \checkmark & \checkmark & \checkmark & \checkmark \\
Herschel/SPIRE & SPIRE/500 & 5111803 & \checkmark & \checkmark & \checkmark & \checkmark & \checkmark \\
\hline
\end{tabular}
\label{tab:candels_bands}
\end{table*}

%\section{MIPS and Herschel limiting fluxes}\label{appB}
%Adopted CANDELS 5$\sigma$ flux density limits for MIPS/24$~\mu$m and Herschel PACS/ 100, 160~$\mu$m, SPIRE/ 250, 350 and 500~$\mu$m (\autoref{tab:IRuppLIM}).
